# Supplementary material for: Lightweight, Secure and Stateful Serverless Computing with PSL
Source: arXiv:2410.20004 source file (2024-10-25)
Supplement: Supplementary file 1 [file appendix.tex]

\pagebreak
\appendix
\section{Proofs of correctness}
\begin{lemma}
\label{lemma:linearizability_proof}
Monotonicity with eventual progress implies linearizability.
\end{lemma}

\noindent \textbf{Proof} (Sketch):
For linearizability to hold, if one worker reads value $V_1$ followed by value $V_2$, no other worker will read value $V_2$ followed by value $V_1$.

If workers follow monotonicity and reads value $V_1$ followed by value $V_2$, we have $V_1 \leq_{e} V_2$.
By eventual progress, every other worker will eventually read values $V_3$ and $V_4$ such that, $V_1 \leq_{e} V_3$ and $V_2 \leq_{e} V_4$.
Without loss of generality, assume $V_3 \leq_{e} V_4$.
Reading $V_3$, then $V_4$ does not break monotonicity.
If the worker reads $V_4$ first, due to monotonicity, it cannot read $V_3$ later.
This also holds when $V_1 = V_3$ and $V_2 = V_4$.
Thus monotonicity with eventual progress implies linearizability.

\begin{lemma}
\label{lemma:correctness_proof}
Under an asynchronous network environment, the protocol described above provides monotonicity, eventual progress, and validity.
\end{lemma}

\noindent \textbf{Proof} (Sketch):
We prove for the case where the working set of keys fit in the workers' Memtables.
The low cache mode discussed above, with pinning, makes the proof easily extensible to smaller Memtable sizes.

For Validity, we note that the writes are proposed by code executing within a TEE.
Outside the TEE, the writes are always encrypted by an AEAD scheme which makes them tamper-proof.
This prevents a malicious adversary from equivocating or injecting malicious writes.

Once a key is inserted in the Memtable, the multicast messages and the Sync Reports merge updates to that key strictly using the $\leq_{e}$ partial order.
We only evict a key if we have received a Sync Report containing the key with the same or greater value (according to $\leq_{e}$) than we have in our Memtable (this is ensured either by having a big enough Memtable or by pinning in the low cache mode).
The next key is read from \Seq, it is guaranteed that the value will be equal to or greater than the value we evicted. This preserves linearizability.

A worker is allowed to miss any number of multicast messages from other workers.
However, the \Seq makes sure of the eventual progress property.
If a worker is alive and constantly proposing new writes, eventually the \Seq will receive a block from the worker.
If the sequence number of the block is $i$, our protocol guarantees that all blocks from the sequence number $1$ to $(i - 1)$ have been replicated to at least $f + 1$ \dcs.
Thus, when it back-fills these blocks, it is guaranteed that at least one \dc will respond with the correct block.
Since the hash of block $(i - 1)$ is attached to block $i$, the \Seq can inductively back-fill all the blocks by querying the hashes.
If the worker has crashed after multicasting a few blocks and the multicast packets have been dropped, these blocks will be visible to the \Seq the next time it checks the blocks from the \dcs.
If the worker crashed before it could replicate the blocks to $f + 1$ \dcs, the key-value pairs in those blocks are not considered as committed by the application.
A properly programmed application should retry these requests using another worker.

\section{Alogrithms for different components}

\begin{algorithm}
\caption{\Dc operation}
\label{alg:dc_op}
\begin{algorithmic}
\State{\textbf{Persistent State:} $storage\_map$: a hashmap containing all writes stored in disk, indexed by the hash $H(.)$ of the block.}
\State{\textbf{In-memory State:} $recent\_block\_map$: list of hashes of the most recent block written by each worker.}

\Function{StoreBlock}{$b, n, sig, worker$} \Comment{Responds to Multicast messages}
\State{$h \leftarrow H(b)$}
\State{$(h^\prime, n^\prime) \leftarrow recent\_block\_map[worker]$}
\If {$n > n^\prime$}
    \State{$recent\_block\_map[worker] \leftarrow (h, n)$}
\EndIf
\State{$storage\_map[h] \leftarrow b$}
\State{\Return{\Call{Ack}{$h$}}}
\EndFunction

\Function{RetrieveBlockByHash}{$h$}
\State{\Return{$storage\_map[h]~ || ~null$ }}
\EndFunction

\Function{RetrieveMostRecentBlock}{$worker$}
\State{$(h, ~\_) \leftarrow recent\_block\_map[worker]$}
\State{\Return{\Call{RetrieveBlockByHash}{$h$}}}
\EndFunction
\end{algorithmic}
\end{algorithm}

\begin{algorithm}
\caption{Worker operation}
\label{alg:worker_op}
\begin{algorithmic}
\State{\textbf{In-memory State:} $Memtable$: a list of $\langle k, V = (v, ts) \rangle$;\\ $n$: current block sequence number;\\ $h$: hash of last block;\\$n_{sr}$: sequence number of the last Sync Report}

\Function{DurableCommit}{$WS = \lbrace \langle k_i, V_i \rangle \forall i \in [1, m]$}
\State{$n \leftarrow n + 1$}
\State{Construct block $b \leftarrow Enc(\langle WS, n, h  \rangle)$} \Comment{AEAD encryption with application key, also signed periodically}
\For{$\langle k_i, V_i \rangle \in WS$}
    \If {$k_i \notin Memtable \vee Memtable[k_i] \leq_{e} V_i$}
        \State{$Memtable[k_i] \leftarrow V_i$}
    \EndIf
\EndFor

\State{$h^\prime \leftarrow H(b)$}
\State{\Call{Multicast}{$b, n$}}
\State{Wait for $f + 1$ replies from \dcs with \Call{Ack}{$h^\prime$}}
\State{$h \leftarrow h^\prime$}
\EndFunction

\Function{HandleMulticast}{$b$}
\State{$(WS, n^\prime, h^\prime) \leftarrow Dec(b)$} \Comment{Decryption fails if block is tampered.}
\For{$\langle k_i, V_i \rangle \in WS$}
    \If {$k_i \notin Memtable \vee Memtable[k_i] \leq_{e} V_i$}
        \State{$Memtable[k_i] \leftarrow V_i$}
    \EndIf
\EndFor
\EndFunction

\Function{HandleSyncReport}{$r$}
\State{$(WS, n^\prime, h^\prime) \leftarrow Dec(r)$} \Comment{Structure of Sync Report described in \Cref{alg:seq_op}.}
\If{$n^\prime > 1 + n_{sr}$}
    \State{$b \leftarrow$ \Call{RetrieveBlockByHash}{$h^\prime$} from any responding \dc}
    \State{\Call{HandleSyncReport}{$b$}} \Comment{Recursively back-fill all missing Sync Reports}
\EndIf
\State{$n_{sr} \leftarrow n^\prime$}
\For{$\langle k_i, (ts_i^\prime, h_i^\prime) \rangle \in WS$}
    \State{($v_i, ts_i) \leftarrow Memtable[k_i]$}
    \If{$ts_i < ts_i^\prime \vee (ts_i = ts_i^\prime \wedge H(v_i) < h_i^\prime)$}
        \State{Delete $k_i$ from $Memtable$ and refresh it from \Seq.}
    \EndIf
\EndFor
\EndFunction

\Function{ReadKey}{$k$}

\If{$k \notin Memtable$}
    \State{Fetch Key from \Seq and store in $Memtable$}
    \State{If \Seq returns the hash pointer to a Checkpoint block, retrieve the block from \dcs and store all keys in $Memtable$.}
\EndIf
\State{\Return{$Memtable[k]$}}

\EndFunction
\end{algorithmic}
\end{algorithm}

\begin{algorithm}
\caption{\Seq operation}
\label{alg:seq_op}
\begin{algorithmic}
\State{\textbf{In-memory State:} $Memtable$: a list of $\langle k, V = (v, ts) \rangle$;\\ $n$: current Sync Report sequence number;\\ $h$: hash of last Sync Report;}
\State{$sorted\_map$: sorted map of all keys to the hash of the Checkpoint block with the most recent update to that key.\\
Only a part of $sorted\_map$ is kept in memory, the rest is stored durably in \dcs.}
\State{$worker\_vc$: A vector clock containing all the workers and their most recent block's sequence number.}

\Function{HandleMulticast}{$b, worker$}
\State{$(WS, n^\prime, h^\prime) \leftarrow Dec(b)$}
\If{$n^\prime > 1 + worker\_vc[worker]$}
    \State{$b^\prime \leftarrow$ \Call{RetrieveBlockByHash}{$h^\prime$}}
    \State{\Call{HandleMulticast}{$b^\prime$}}
\EndIf
\State{$worker\_vc[worker] \leftarrow n^\prime$}
\For{$\langle k_i, V_i \rangle \in WS$}
    \If {$k_i \notin Memtable \vee Memtable[k_i] \leq_{e} V_i$}
        \State{$Memtable[k_i] \leftarrow V_i$}
    \EndIf
\EndFor
\EndFunction

\Function{Checkpoint}{}
\For{$worker \in worker\_vc$}
\State{Call \Call{RetrieveMostRecentBlock}{$worker$} and wait for $(n - f)$ responses.}
\State{Let $n^\prime$ be the highest sequence number received for $worker$}
\If {$n^\prime > worker\_vc[worker]$}
    \State{\Call{HandleMulticast}{$b^\prime, worker$}, where $b^\prime$ is the block corresponding to $n^\prime$}
\EndIf

\State{$n \leftarrow n + 1$}

\State{Construct Checkpoint $chkpt \leftarrow \langle Memtable, n \rangle$}
\State{\Call{Multicast}{$Enc(chkpt)$} only to \dcs.}
\State{$h_{chkpt} \leftarrow H(Enc(chkpt))$}
\State{Wait for $f + 1$ responses with \Call{Ack}{$h_{chkpt}$}}

\State{Construct $WS \leftarrow \lbrace \langle k_i, (ts_i, H(v_i)) \rangle \forall k_i \in Memtable \rbrace$}

\State{Construct Sync Report $r \leftarrow Enc(\langle WS, n, h \rangle$)}
\State{$h \leftarrow H(r)$}
\State{\Call{Multicast}{$r$} to all workers and \dcs.}
\State{Wait for $f + 1$ responses with \Call{Ack}{$h$}}

\State{$sorted\_map[k_i] \leftarrow h_{chkpt} ~\forall k_i \in Memtable$}
\State{Flush $Memtable$}

\EndFor
\EndFunction

\Function{FetchKey}{$k$}
\If{$k \in Memtable$}
    \State{\Return{$Memtable[k]$}}
\Else
    \State{\Return{$sorted\_map[k]$}} \Comment{This returns the hash of the Checkpoint block that stores the most recent version of $k$ as seen by \Seq}
\EndIf
\EndFunction
\end{algorithmic}
\end{algorithm}
